# Supplementary material for: Efficient Visual Computing with Camera RAW Snapshots
Source: arXiv:2212.07778 source file (2024-01-25)
Supplement: Supplementary file 1 [file supp_hardware_results.tex]

\begin{figure}[t]
\centering
\includegraphics[width=1.0\linewidth]{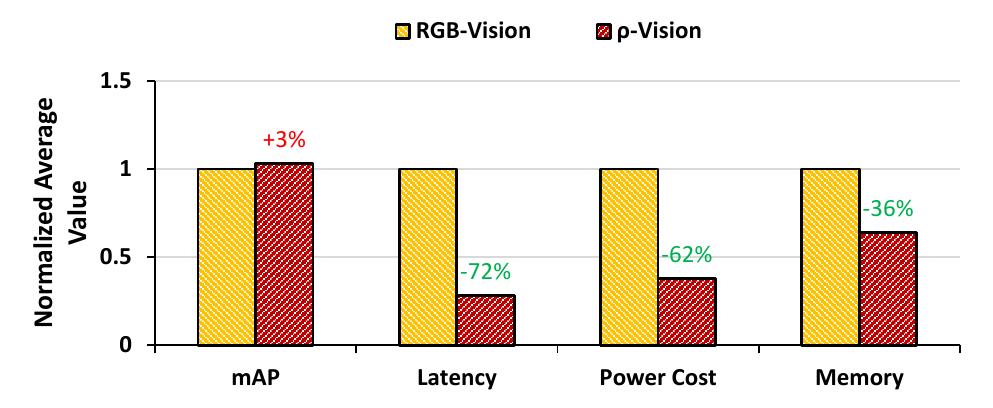}
%\end{center}
\caption{{\bf Normalized Average Gains for $\rho$-Vision Compared to RGB-Vision.} Metrics are normalized to RGB-Vision framework evaluation results, with the mAP scores tested from multiRAW (iPhone RAW) detection tasks. Latency refers to the total time consumption of the entire pipeline, power cost is measured using a power meter, and memory usage is monitored during operation.}
\label{fig:supp_hardware_results}
\end{figure}
