# Supplementary material for: Efficient Visual Computing with Camera RAW Snapshots
Source: arXiv:2212.07778 source file (2024-01-25)
Supplement: Supplementary file 2 [file supp_ablation_gamma.tex]

\begin{table*}
    \small
    \setlength{\tabcolsep}{5.5pt}
    \centering
    \caption{Impact of Gamma Correction (GC) on segmentation.}
    \label{table:supp_ablation_gamma}
    \begin{threeparttable}
    \begin{tabular}{lccccccccccccc}
    \toprule
    \textbf{Domain} & 
    \textbf{Road} &
    \textbf{Building} &
    \textbf{Fence} &
    \textbf{Tr. Light} &
    \textbf{Tr. Sign} &
    \textbf{Plant} &
    \textbf{Sky} &
    \textbf{Person} &
    \textbf{Car} &
    \textbf{Truck} &
    \textbf{Bus} &
    \textbf{Bicycle} &
    \textbf{mIoU} \\ \midrule
    RGB &
    \textbf{91.7} &
    81.6 &
    \textbf{56.4} &
    39.2 &
    \textbf{73.5} &
    \textbf{92.2} &
    95.1 &
    \textbf{34.3} &
    \textbf{66.3} &
    \textbf{55.8} &
    \textbf{68.7} &
    \textbf{47.2} &
    \textbf{66.8} \\
    RAW w/o GC &
    35.8 &
    44.2 &
    20.0 &
    9.7 &
    14.8 &
    42.4 &
    95.8 &
    14.4 &
    20.9 &
    9.1 &
    35.7 &
    12.7 &
    29.6 \\
    RAW w/ GC &
    89.3 &
    \textbf{83.2} &
    56.1 &
    \textbf{40.2} &
    70.9 &
    91.2 &
    \textbf{96.9} &
    34.0 &
    65.8 &
    48.1 &
    63.6 &
    41.4 &
    65.0 \\
    \bottomrule
    \end{tabular}
    
    \begin{tablenotes}
        \footnotesize 
        \item \textbf{Tr. Light} $\leftarrow$ Traffic Light; \textbf{Tr. Sign} $\leftarrow$ Traffic Sign.
    \end{tablenotes}
    
    \end{threeparttable}
    
\end{table*}
